# Supplementary material for: Information flow at the quantum-classical boundary
Source: arXiv:0901.3629 source file (2009-01-23)
Supplement: Supplementary file 1 [file thesis-appendix.tex]

%\chapter{Sampling theory with C$^*$-algebras}

%There exists a generalization of sampling theory which uses the concept of self-adjoint extension of unbounded operators. Here we show how these results can be reformulated, and maybe generalized, in the language of C$^*$-algebras. 
